# Supplementary material for: Re-evaluating Group Robustness via Adaptive Class-Specific Scaling
Source: arXiv:2412.15311 source file (2024-12-19)
Supplement: Supplementary file 1 [file prelim_supple.tex]

 % !TEX root = ../main.tex
 
% 
% \section{Preliminaries}
% \label{sec:prelim}
%
% \subsection{Problem Setup}
% Let consider a triplet $(x, y, a)$ consisting of an input feature $x \in \mathcal{X}$, a target label $y \in \mathcal{Y}$, and a spurious attribute $a \in \mathcal{A}$. 
% We define the group as a pair of target label and spurious attribute, $g := (y, a) \in \mathcal{Y} \times \mathcal{A} =: \mathcal{G}$.
% We are basically given $n$ training examples without group annotations, \eg, $\{(x_1, y_1), ..., (x_n, y_n)\}$, while given $m$ validation examples with group annotations for model selection, \eg, $\{(x_1, g_1), ..., (x_m, g_m)\}$ = $\{(x_1, y_1, a_1), ..., (x_m, y_m, a_m)\}$.
% 
%% \begin{align}
%%     \text{UA} := \frac{1}{N}\sum_{i=1}^N \mathbf{1}(f_\theta(\mathbf{x}_i) = y_i )
%% \end{align}
% Our goal is to learn a model $f_\theta(\cdot): \mathcal{X} \rightarrow \mathcal{Y}$ that is robust to group distribution shifts.
%%  To evaluate the group robustness, let first define the group-wise accuracy (GA).
% To measure the group robustness, unbiased accuracy (UA) and worst-group accuracy (WA) are usually adopted.
% Let first define the group-wise accuracy (GA):
% \begin{align}
%    \text{GA}_{(r)} := \frac{\sum_{i} \mathds{1}(f_\theta(\mathbf{x}_i) = y_i, g_i=r)}{\sum_{i} \mathds{1}(g_i=r)},
%\end{align}
%where $\mathds{1}(\cdot)$ is an indicator function and $\text{GA}_{(r)}$ denotes the accuracy of $r^\text{th}$ group samples.
%Unbiased and worst-group accuracies are defined by
%\begin{align}
%    \text{UA} := \frac{1}{|\mathcal{G}|}\sum_{r\in\mathcal{G}}{\text{GA}_{(r)}},~~~~~ \text{WA} := \max_{r\in\mathcal{G}} \text{GA}_{(r)},
%\end{align}
%both of which are also referred to as robust accuracy.
% 
% \subsection{Comparisons} 
%%Below is a brief introduction of the comparisons used in our experiments.
%
% \paragraph{ERM}
% Given a loss function $\ell(\cdot)$, the objective of empirical risk minimization is optimizing the following loss over training data: 
% \begin{align}
%    %  \min_\theta \Big\{ \mathcal{L}_\text{ERM}(f_\theta) := \mathbb{E}_{(x,y,a)\sim P}[\ell(f_\theta(x), y)] \Big\}
%    \min_\theta \Big\{\frac{1}{n}\sum_{i=1}^n \ell(f_\theta(x_i), y_i) \Big\}.
% \end{align}
%%  where $P$ is the empirical distribution over training data.
% 
% \paragraph{Class reweighting (CR)}
% To mitigate the class imbalance issue, we can simply reweight the samples based on the inverse of class frequency in the training split, 
%  \begin{align}
%    \min_\theta \Big\{\frac{1}{n}\sum_{i=1}^n \omega_i \ell(f_\theta(x_i), y_i) \Big\}~~\text{where}~~\omega_i = \frac{n}{\sum_j \mathds{1}(y_j=y_i)}
% \end{align}
% 
% \paragraph{LfF}
%Motivated by the observation that bias-aligned samples are more easily learned, LfF~\citep{LfF} simultaneously trains a pair of neural network $(f_B, f_D)$.
%The biased model $f_B$ is trained with generalized cross-entropy loss which intends to amplify bias, while the debiased model $f_D$ is trained with a standard cross-entropy loss, where each sample $(x_i, y_i)$ is reweighted by the following relative difficulty score:
%\begin{align}
%%    \omega_i = \frac{\log f_B(y_i|x_i)}{\log f_B(y_i|x_i) + \log f_D(y_i|x_i)}.
%    \omega_i = \frac{\ell(f^B_\theta(x_i), y_i)}{\ell(f^B_\theta(x_i), y_i) + \ell(f^D_\theta(x_i), y_i)}.
%\end{align}
%
% 
%
% \paragraph{JTT}
% JTT~\citep{JTT} consists of two-stage procedures. In the first stage, JTT trains a standard ERM model $\hat{f}(\cdot)$ for several epochs and identifies an error set $E$ of training examples that are misclassified:
% \begin{align}
%E := \{(x_i, y_i)~~\text{s.t.}~\hat{f}(x_i) \neq y_i \}.
% \end{align}
% Next, they train a final model $f_\theta(\cdot)$ by upweighting the examples in the error set $E$ as
% \begin{align}
%      \min_\theta \Big\{  \lambda_\text{up}\sum_{(x,y)\in E}\ell(f_\theta(x), y) + \sum_{(x,y)\notin E}\ell(f_\theta(x), y) \Big\}.
% \end{align}
% 
% 
% 
% \paragraph{Group DRO}
%%  While ERM is the standard way and generally works well, it often learns spurious correlation and consequently, it leads to poor robust accuracy.
%%  To tackle this problem, Group DRO aims to minimize the worst-group loss formulated as:
%Group DRO~\citep{GroupDRO} aims to minimize the empirical worst-group loss formulated as:
% \begin{align}
%  \min_\theta \Big\{
%     \max_{g\in \mathcal{G}} \frac{1}{n_g} \sum_{i|g_i=g}^{n_g} \ell(f_\theta(x_i), y_i) \Big\}
% \end{align}
% where $n_g$ is the number of samples assigned to $g^\text{th}$ group.
% Unlike previous approaches, group DRO requires group annotations $g=(y,a)$ on the training split.
%%  Unlike Group DRO, we basically assume that we do not have group annotations in training data, and we are only given a small validation set with group annotations.
%
%\paragraph{Group reweighting (GR)}
% Using group annotations, we can extend class reweighting method to group reweighting one based on the inverse of group frequency in the training split, \ie,
%%  $\omega_i = n/{\sum_j \mathds{1}(y_j=y_i, a_j=a_i)}$.
%   \begin{align}
%    \min_\theta \Big\{\frac{1}{n}\sum_{i=1}^n \omega_i \ell(f_\theta(x_i), y_i) \Big\}~~\text{where}~~ \omega_i = \frac{n}{\sum_j \mathds{1}(y_j=y_i, a_j=a_i)}
%  \end{align}
% 
